# Supplementary material for: Uncovering Biases with Reflective Large Language Models
Source: arXiv:2408.13464 source file (2024-10-24)
Supplement: Supplementary file 1 [file AppendicD.tex]

\documentclass[11pt,fleqn]{article}
\usepackage{longtable}
\usepackage{etoolbox}
\usepackage{booktabs}       % professional-quality tables
\usepackage{tikz}
\usepackage{tabularx}
\usepackage{comment}
\usepackage{enumitem}
\usepackage{amsmath}
\usepackage{amsfonts}
\usepackage{hyperref}
\setlength{\mathindent}{6pt} % Adjusts the indentation of the left-aligned equations
\pagestyle{plain}
\usepackage{amssymb}
\usepackage{algorithm}
\usepackage{algorithmic}
\usepackage{marvosym}
\usepackage{balance}
\usepackage{flushend}

\begin{document}
    
\section*{Response to Previous Round of Reviewers}

This paper received a 3.5, 3, and 3 review in the last ACL cycle. The area chair decided to reject the paper with three reasons. 

\begin{enumerate}[leftmargin=1.2em, topsep=.1em, parsep=.1em, label=\arabic*.]
\item Notable aspects of the approach have been published in (anonymized) prior work already. As a result, a lot of information has been outsourced to references and an appendix found online. In the response, the authors further point to more anonymous sources found online, which in my view is all not really ideal. I understand that building upon own previous work in an anonymous way is not easy, but it's also a common problem in our community. I would suggest to make the paper as self-contained as possible and to clarify explicitly what is new to the submission itself.
\item The paper lacks a comparison to baseline approaches to bias mitigation, which leaves unclear how the good the obtained results really are. While it's not at the core of the intended contribution to beat SOTA approaches, such comparisons may still help interpret the results observed.
\item The data has been annotated by one annotator from each political side only. This may introduce the individual biases of the respective people into the approach itself and should be discussed clearly in the paper.
\end{enumerate}

\paragraph{Response:}
Our extensive enhancements and answers are as follows:
\newline
\begin{enumerate}[leftmargin=1.2em, topsep=-.2em, parsep=-.4em, label=\arabic*.]
\item \textit{Contributions Unclear with Several Anonymous Pointers}:
While we acknowledge the challenge of providing definitive evidence for priority in anonymous submissions, we have followed the reviewer's suggestion to make this revision self-contained. This revision substantially enhances the previous version by incorporating a comprehensive theoretical foundation, including seven maxims, a novel theory (entropy duality), and multiple quality metrics. These additions enable us to monitor information exchange progress (mutual information), measure debate convergence (Wasserstein distance, cross-entropy, Jensen-Shannon divergence), and establish the optimal conditions for achieving high-quality results. We believe this expanded theoretical grounding and enhanced transparency significantly strengthen the contribution of our work. \\
\item \textit{Baseline Comparisons for EVINCE}:
Regarding the question of a baseline for comparison, it is important to note that, to the best of our knowledge, no existing white-box schemes aim to correct erroneous or biased ground-truth annotations directly. EVINCE represents a novel approach in this domain. Most existing methods focus on model adjustments rather than the foundational issue of annotation bias. Thus, EVINCE's unique contribution lies in its proactive correction of biased ground-truths, setting a new standard in bias mitigation. Comparisons with standard annotation practices or black-box methods would not provide a meaningful benchmark due to the fundamentally different objectives and methodologies. \\
\item \textit{Mitigating Annotation Bias by Adding More Annotators}:
The concern regarding whether adding more annotators could mitigate annotation bias is addressed by our methodology. Reported by [1], the annotators were randomly selected from a pool of 749 qualified individuals (each must be a US resident, but have a 98+\% Amazon Turk credential, and must be knowledgeable about political subjects), ensuring a statistically representative sample of both Republican-leaning and Democrat-leaning perspectives. This random selection process is designed to effectively mitigate individual biases. Given the size, quality, and representativeness of the pool, adding more annotators is not expected to alter the statistical robustness of our findings. \\
\newline
Furthermore, adding more annotators, such as additional Republican-leaning ones, might better characterize an average Republican-leaning annotator's bias, but that is not the aim of this paper. Biases are unavoidable in our increasingly polarized society on various subjects. This paper focuses on how these biases can be identified and mitigated. Therefore, we stand by our approach as both rigorous and sufficient to address potential annotation biases.
\end{enumerate}

\paragraph{Dataset Description (added to Section 4.1):}

The dataset for this experiment consists of 619 news articles (54.3\% about Democrat scandals, 45.7\% about Republican scandals) selected from a larger 2013 repository of 14,033 articles compiled by fifteen reputable news organizations [1]. These articles cover diverse topics such as civil rights, healthcare, elections, and national security. This dataset is provided as supplementary material. \\
\newline
The articles were originally labeled through Amazon Mechanical Turk by 749 qualified U.S. workers, each annotating up to 1,000 randomly selected articles [1]. Each worker was qualified through three criteria: U.S. residence, knowledge of political news, and being an experienced Amazon Turk worker with a 98+\% rating. For each ``scandal'' article in our subset, one Democrat and one Republican annotator independently classified its bias as ``negatively biased,'' ``weak negative,'' ``neutral," ``weak positive,'' or ``positively biased.'' \\
\newline
This subset is valuable due to its ground-truth labels provided by annotators from opposing political affiliations, revealing inherent biases in evaluating negative coverage of one's own party. The original study [1] found that Republican annotators often perceive news about Republican scandals as negatively biased, while Democrat annotators tend to view such news as neutral or "just right," potentially indicating satisfaction with the coverage's perceived fairness.

\bibliographystyle{plain}
\bibliography{References-1,References-2,SocraPedia,Evince}

[1] Ceren Budak, Sharad Goel, and Justin M. Rao. 2016. 687 Fair and Balanced? Quantifying Media Bias through 688 Crowdsourced Content Analysis. Public Opinion 689 Quarterly, 80(S1):250–271.

\end{document}
