# Supplementary material for: Uncovering Biases with Reflective Large Language Models
Source: arXiv:2408.13464 source file (2024-10-24)
Supplement: Supplementary file 2 [file AppendixC_D.tex]

\begin{comment}
 
\section*{Appendix B: Wikipedia Content Ratings}

\begin{itemize}[left=0em]
\item Featured (FA and FL): Represents the pinnacle of quality, either as a featured article or list, showcasing comprehensive coverage and exceptional standards.
\item A: An excellent article that hasn't undergone the full review process for 'Featured' status but is nonetheless well-organized, complete, and reliably sourced.
\item GA and B-class: Articles that are well-crafted ('Good Article') or fairly well written (B-class), with appropriate references and adherence to Wikipedia's guidelines.
\item C-class: A significant article with notable gaps in content or inclusion of irrelevant material, having some but potentially insufficient references.
\item Start: An article in its developmental stages, characterized by incompleteness and likely poor organization.
\item Stub-class: The most basic form of content, and requiring extensive development.
\end{itemize}
   
\end{comment}
\section*{Appendix B: Experiment \#2, Debate \#2}

Table~\ref{tab:Quantum-Debate} provides an overview of the discussion surrounding the proposition: ``{\em Quantum entanglement} has the potential to significantly transform the fields of computing and artificial intelligence.'' This debate is particularly pertinent given the escalating excitement and, occasionally, the excessive hype associated with quantum computing's capabilities and future impact. By engaging in this debate, we aim to critically evaluate and place the potential of quantum entanglement in computing and artificial intelligence into an accurate and measured perspective.

The structure of the debate is delineated through the participation of two distinct agents. Agent 1 assumes the role of the proponent, advocating for the transformative power of quantum entanglement in revolutionizing computing and artificial intelligence. In contrast, Agent 2 adopts a skeptical stance, challenging the optimistic projections and questioning the current state and near-future possibilities offered by quantum technologies.

%The arguments and counterarguments put forth by each agent are methodically cataloged in the table, providing readers with a clear and direct comparison of the viewpoints. This structured presentation facilitates an in-depth understanding of the diverse perspectives on quantum entanglement's role in future technological advancements. Following the exchange of ideas, the table concludes with a summary of each agent's final stance, encapsulating the essence of their arguments and the implications for the field of quantum computing and artificial intelligence.

%This detailed debate format aims to illuminate the complexities and nuances associated with quantum entanglement and its applicability to computing and AI, moving beyond simplistic narratives to foster a more informed discussion within the scientific community.

\begin{table*}[ht!]
%\begin{small}
\centering
\begin{tabular}{|p{8.0cm}|p{7.3cm}|}
\toprule
\hline
{Agent \#1 Supporting Arguments} & {Agent \#2 Opposing Arguments} \\ \hline
\hline
{\begin{enumerate}[leftmargin=1.2em, topsep=-.2em, parsep=-.4em, label=\arabic*.]
\item My key arguments center around several significant aspects and developments. These include empirical evidence proving \textit{quantum entanglement} through experiments like Bell's Theorem, the immense potential and emerging breakthroughs of quantum computing (e.g., Google's Sycamore processor), the possible transformative effects on AI, the inception of revolutionary quantum algorithms, the prospects of quantum networks, quantum enhancement of data security through unbreakable encryption, and the potential for birthing new quantum-based technologies.

\item While recognizing the concerns raised by Agent2 about experimental limitations, the challenges in erecting scalable, efficient quantum computers, hurdles in quantum error correction and AI integration, the limitations of existing quantum algorithms, infrastructure and training obstacles, and skepticism about the extent of the quantum revolution, I have drawn attention to the ongoing efforts and substantial progress in these areas. 

\item For instance, experimental entanglement has been successfully demonstrated despite their controlled settings, large strides are being made in the scalability and efficiency of quantum computers, error correction methodologies are being developed and refined, Quantum Machine Learning heralds a promising intersection of quantum computing and AI, and new quantum algorithms are an active area of research.
\item A marked difference between Agent2 and me lies in our outlook towards the future of \textit{quantum entanglement}. While both of us acknowledge the challenges, I express robust optimism.
\end{enumerate}}
&
{
\begin{enumerate}[leftmargin=1.2em, topsep=-.2em, parsep=-.4em, label=\arabic*.]
\item The central arguments for my stance include experimental uncertainties, quantum computing hurdles, a high quantum error rate, the challenges with incorporating quantum computing into AI, the early stage of quantum algorithms, and the demands on infrastructure and human resources.

\item These counterpoints refute many of Agent1's affirmations. Despite the scientific proof of \textit{quantum entanglement}, it's essential to understand that these proofs come from controlled lab environments, often wrestling with loopholes and scalability issues. While Google's demonstration of quantum supremacy showcases the potential, it does not invalidate the fact that quantum computers, as of now, are delicate, error-prone and largely inefficient compared to classical ones. 

\item Concerning AI, while theoretically, quantum computing could indeed provide benefits, current AI systems are fully entrenched in classical computing. Moreover, the inherent instability and error-proneness of quantum computing currently make them less suitable for AI tasks that rely on vast amounts of real-world data.

\item Significant differences exist between our positions. While Agent1 seems eager to champion the potential of quantum technology, I lean towards a more cautious and practical assessment, highlighting the significant hurdles we currently face in making quantum computing and AI a reliable, efficient reality.
\end{enumerate}} \\ \hline

{In summary, our debate has provided a comprehensive overview of the fascinating realm of \textit{quantum entanglement}, its potential impact on computing and AI, and the associated challenges. It is clear that we are at the cusp of a quantum revolution, albeit faced with substantial hurdles. While the speed and scope of this change remain open questions, the sheer potential of \textit{quantum entanglement} makes it an exciting field to watch as we venture into the quantum era. } & 
{In summary, the future of \textit{quantum entanglement} in computing and AI is still uncertain with numerous unresolved issues. These include developing stable, practical quantum computers, creating quantum algorithms applicable to a broad range of problems, and successfully integrating quantum computing into classical systems and AI. It is crucial not to overlook the vast scientific and practical challenges that precede it. }
\\ \hline
\bottomrule
\end{tabular}
%\end{small}
\caption{Debate subject: \textit{Quantum entanglement} holds tremendous potential to revolutionize computing and advance artificial intelligence?}
\label{tab:Quantum-Debate}
\end{table*}

\section*{Appendix C: Training Dataset}

The training dataset used in Section 5 were
submitted on Open Review under the Data section.  
The link provided in reference \cite{SocraSynthBiasesDataSet} 
can also access the dataset.

\section*{Appendix Z: Additional Supplementary Materials}

For additional experimental results, datasets, and 
debate interactions, please refer to our supplementary
materials \cite{ACLSupplementary}.
