# Supplementary material for: Uncovering Biases with Reflective Large Language Models
Source: arXiv:2408.13464 source file (2024-10-24)
Supplement: Supplementary file 3 [file AppendixE-EthicalStatement.tex]

\section*{Ethical Statements}

This research, conducted in alignment with the Association for Computational Linguistics' ethical guidelines, primarily aims to mitigate fairness and biases in computational linguistics and to address the challenges of inaccurate and biased information. We have not involved any direct human or animal subjects in our study. All data utilized for computational analysis is sourced from publicly available datasets or collected with explicit consent, respecting privacy and data protection standards.

We have implemented rigorous measures to anonymize any sensitive data to safeguard individual privacy. Our algorithms are specifically designed to promote fairness, actively working to identify and rectify biases with LLMs. Additionally, this study contributes to the detection and correction of inaccurate and misleading information, a crucial step towards ensuring the integrity and reliability of data in natural language processing.

We acknowledge the potential impact of our research, especially in the context of misinformation and bias in AI technologies. Our commitment is to foster advancements in the field that are both ethically responsible and socially conscious, acknowledging the significant role these technologies play in shaping public discourse and information dissemination.

In the execution of this project, we utilized GPT-4, specifically for the purposes of conducting multi-LLM debates and providing editorial assistance. Apart from these specified uses, no artificial intelligence tools were employed in any other aspects of this work's completion.
