# Supplementary material for: Uncovering Biases with Reflective Large Language Models
Source: arXiv:2408.13464 source file (2024-10-24)
Supplement: Supplementary file 4 [file ACLSupplementary.tex]

% This must be in the first 5 lines to tell arXiv to use pdfLaTeX, which is strongly recommended.
\pdfoutput=1
% In particular, the hyperref package requires pdfLaTeX in order to break URLs across lines.

\documentclass[11pt,fleqn]{article}

% Remove the "review" option to generate the final version.
%\usepackage[review]{acl}
\usepackage[review]{acl}

% Standard package includes
\usepackage{times}
\usepackage{latexsym}

% For proper rendering and hyphenation of words containing Latin characters (including in bib files)
\usepackage[T1]{fontenc}
% For Vietnamese characters
%\usepackage[T5]{fontenc}
% See https://www.latex-project.org/help/documentation/encguide.pdf for other character sets

% This assumes your files are encoded as UTF8
%\usepackage[utf8]{inputenc}

% This is not strictly necessary, and may be commented out,
% but it will improve the layout of the manuscript,
% and will typically save some space.
\usepackage{microtype}

% This is also not strictly necessary, and may be commented out.
% However, it will improve the aesthetics of text in
% the typewriter font.
%\usepackage{inconsolata}
%\usepackage{amsmath,amssymb,amsfonts}
%\usepackage{algorithmic}
%\usepackage{graphicx}
%\usepackage{textcomp}
%\usepackage{xcolor}
%\def\BibTeX{{\rm B\kern-.05em{\sc i\kern-.025em b}\kern-.08em
%    T\kern-.1667em\lower.7ex\hbox{E}\kern-.125emX}}

%-------------------------------- 0210
%\usepackage[english]{babel}
%\usepackage[square,numbers]{natbib}
\usepackage{longtable}
\usepackage{etoolbox}
\usepackage{booktabs}       % professional-quality tables
\usepackage{balance}
\usepackage{tikz}
\usepackage{tabularx}
\usepackage{comment}
\usepackage{enumitem}
\usepackage{amsmath}
\usepackage{amsfonts}
\usepackage{hyperref}
\setlength{\mathindent}{6pt} % Adjusts the indentation of the left-aligned equations

\title{It Takes a Mirror to Find Flaws: Uncovering Biases with Reflective Large Language Models (Supplementary Materials)}

% Author information can be set in various styles:
% For several authors from the same institution:
% \author{Author 1 \and ... \and Author n \\
%         Address line \\ ... \\ Address line}
% if the names do not fit well on one line use
%         Author 1 \\ {\bf Author 2} \\ ... \\ {\bf Author n} \\
% For authors from different institutions:
% \author{Author 1 \\ Address line \\  ... \\ Address line
%         \And  ... \And
%         Author n \\ Address line \\ ... \\ Address line}
% To start a separate ``row'' of authors use \AND, as in
% \author{Author 1 \\ Address line \\  ... \\ Address line
%         \AND
%         Author 2 \\ Address line \\ ... \\ Address line \And
%         Author 3 \\ Address line \\ ... \\ Address line}

\author{Edward Y. Chang \\
  Computer Science, Stanford University \\
  \texttt{echang@cs.stanford.edu} 
  }

\AtBeginDocument{%
  \setlength{\abovedisplayskip}{3pt plus 1pt minus 1pt} % Space above equation
  \setlength{\belowdisplayskip}{3pt plus 1pt minus 1pt} % Space below equation
  \setlength{\abovedisplayshortskip}{1pt plus 1pt minus 1pt} % Space above equation if preceded by a short line
  \setlength{\belowdisplayshortskip}{1pt plus 1pt minus 1pt} % Space below equation if followed by a short line
}
\begin{document}
\maketitle
%\noindent
%\input{Introduction}
%\input{WikiUsageChallenges}
%\input{SocraPedia}
%\input{SocraSynth}
%\input{CaseStudy} % Section 5
%\input{Conclusion}

\input{AppendixA}
\renewcommand*{\bibfont}{\footnotesize}
\bibliography{References-1,References-2,SocraPedia}
\input{AppendixB_C}
\input{AppendixZ}
\end{document}
